# Supplementary material for: Dynamics of spatial phase coherence in a dissipative Bose-Hubbard atomic system
Source: arXiv:2405.03226 ancillary file (2024-05-07)
Supplement: Supplementary file 1 [file Supplemental_Information.pdf]

# Dynamics of spatial phase coherence in a dissipative Bose-Hubbard atomic system: details of calculations


Rémy Vatré,[1] Raphaël Bouganne,[1] Manel Bosch Aguilera,[1] Alexis Ghermaoui,[1] Jérôme Beugnon,[1] Raphael Lopes,[1] and Fabrice Gerbier[1,*]

[1] *Laboratoire Kastler Brossel, Collège de France, CNRS, ENS-Université PSL, Sorbonne Université, 11 place Marcelin Berthelot, F-75231 Paris, France*



(Dated: May 6, 2024)


## I. ANALYSIS OF THE DISSIPATIVE BOSE-HUBBARD MODEL

In this Section, we give the details of the theoretical analysis of the dissipative Bose-Hubbard model (DBHM) proposed by Poletti *et al.* [1, 2]. We summarize their methods and results for the sake of completeness. We consider a lattice of $N_s$ sites in one dimension (for simplicity) and introduce a vector of occupation numbers $\boldsymbol{n} = (n_1, \cdots, ..., n_{N_s})^T$ to identify a particular Fock state configuration. Using Eqs. (10-12) in the main article, one finds that the components $\rho^{\boldsymbol{n}}_{\boldsymbol{m}} = \langle \boldsymbol{n}|\hat{\rho}|\boldsymbol{m}\rangle$ of the density matrix in the Fock basis obey a set of coupled equations,

$$\frac{d}{dt}\rho^{\boldsymbol{n'}}_{\boldsymbol{n}} = \left(\frac{\Delta E(\boldsymbol{n'},\boldsymbol{n})}{\mathrm{i}\hbar} - \frac{\gamma_{\rm sp}}{2}\left|\boldsymbol{n}-\boldsymbol{n'}\right|^2\right)\rho^{\boldsymbol{n}'}_{\boldsymbol{n}} + \frac{\mathrm{i}\,J}{\hbar}\sum_{\boldsymbol{m}}\left[\langle \boldsymbol{n'}|\hat{T}|\boldsymbol{m}\rangle\rho^{\boldsymbol{m}}_{\boldsymbol{n}} - \langle \boldsymbol{m}|\hat{T}|\boldsymbol{n}\rangle\rho^{\boldsymbol{n'}}_{\boldsymbol{m}}\right]. \tag{1}$$

The two terms inside the parenthesis in the right hand side (rhs) of Eq. (1) come respectively from the interaction Hamiltonian and the dissipator, both local in the Fock basis. The interaction term describes the precession of the phase of the off-diagonal elements $\rho^{\boldsymbol{n'}}_{\boldsymbol{n}}$ at the Bohr frequency $\Delta E(\boldsymbol{n'},\boldsymbol{n}) = \frac{U}{2}\sum_i\left(n'_i(n'_i-1)-n_i(n_i-1)\right)$. The dissipative term is proportional to the distance in Fock space between the two configurations defined as $|\boldsymbol{n}-\boldsymbol{n'}| = \sqrt{\sum_i (n_i-n'_i)^2}$. The form of the dissipator implies that a superposition of two Fock state decays rapidly to a statistical mixture, and that the decay rate increases quadratically with the distance. Finally, the last two terms in the rhs of Eq. (1) describe the build-up by coherent tunnelling of coherences of the form $\rho^{\boldsymbol{n}+\boldsymbol{e}_{i,j}}_{\boldsymbol{n}}$, where the vector $\boldsymbol{e}_{i,j}$ has components $(\boldsymbol{e}_{i,j})_k = \delta_{ik}-\delta_{jk}$ and where $i,j$ are nearest-neighbors.

Taking $\boldsymbol{m}=\boldsymbol{n}$ in the general formula (1), we obtain the evolution of the Fock state populations $\pi_{\boldsymbol{n}} \equiv \rho^{\boldsymbol{n}}_{\boldsymbol{n}}$,

$$\frac{d\pi_{\boldsymbol{n}}}{dt} = -\frac{J}{\mathrm{i}\hbar}\sum_{i,\sigma=\pm1}\sqrt{n_i(n_{i+\sigma}+1)}\left(\rho^{\boldsymbol{n}+\boldsymbol{e}_{i+\sigma,i}}_{\boldsymbol{n}} - \rho^{\boldsymbol{n}}_{\boldsymbol{n}+\boldsymbol{e}_{i+\sigma,i}}\right). \tag{2}$$

The local term vanishes identically, and the populations evolve only by coupling to the "nearest-neighbor coherences" $\rho^{\boldsymbol{n}+\boldsymbol{e}_{i\pm1,i}}_{\boldsymbol{n}}$, *i.e.* coherences between two Fock states differing only by a particle-hole pair on neighboring sites.

We consider next the evolution of the coherences of the form $\rho^{\boldsymbol{n}+\boldsymbol{e}_{i+s,i}}_{\boldsymbol{n}}$. We will refer to such a coherence $\rho^{\boldsymbol{m}}_{\boldsymbol{n}}$ as a coherence of order $s=|i-j|$ if $\boldsymbol{m}-\boldsymbol{n}=\boldsymbol{e}_{i,j}$ for some pair $i,j$. We have

$$\frac{d}{dt}\rho^{\boldsymbol{n}+\boldsymbol{e}_{i+s,i}}_{\boldsymbol{n}} \approx -\lambda_{i+s,i}\rho^{\boldsymbol{n}+\boldsymbol{e}_{i+s,i}}_{\boldsymbol{n}} - \frac{J}{\mathrm{i}\hbar}S_{i+s,i}(t). \tag{3}$$

Here we defined the characteristic complex frequency $\lambda_{i+s,i} = \gamma_{\rm sp} + \mathrm{i}\frac{U}{\hbar}\left(n_{i+s}-n_i+1\right)$ and a "source term"

$$S_{i+s,i} = \langle \boldsymbol{n}+\boldsymbol{e}_{i+s,i}|\left[\hat{T},\hat{\rho}\right]|\boldsymbol{n}\rangle. \tag{4}$$

Eq. (3) can be integrated formally,

$$\rho^{\boldsymbol{n}+\boldsymbol{e}_{i+s,i}}_{\boldsymbol{n}}(t) = \rho^{\boldsymbol{n}+\boldsymbol{e}_{i+s,i}}_{\boldsymbol{n}}(0)\mathrm{e}^{-\lambda_{i+s,i}t} - \frac{J}{\mathrm{i}\hbar}\int_0^t S_{i+s,i}(t-\tau)\mathrm{e}^{-\lambda_{i+s,i}\tau}d\tau. \tag{5}$$


* fabrice.gerbier@lkb.ens.fr

The source term $S_{i+s,i}$ involves contributions from all coherences of order $s-1$ and $s+1$ (its explicit expression is rather massive and uninspiring). The dynamical equations thus generates a chain where populations are coupled to $s=1$ coherences, themselves coupled to populations and to $s=2$ coherences, etc. This structure, often encountered in the density matrix formulation of quantum mechanics, is generally untractable exactly. To handle the problem, we need an approximation scheme that allows us to truncate the chain at a low order.

To that end, Poletti *et al.* [1] remarked that in a system where single-particle correlations are short-ranged, the density matrix is essentially diagonal in the Fock basis, with small off-diagonal coherences that become smaller the further away they are from the diagonal. In other words, populations are much larger than coherences with $s=1$, themselves much larger than coherences with $s=2$, etc. As a result, we may approximate the "source" term $S_{i+s,i}$ that drives the evolution of the coherence of order $s$ by keeping only the dominant contribution of coherences of order $s-1$, *i.e.* $\rho_{\boldsymbol{n}}^{\boldsymbol{m}}$ with $(\boldsymbol{n},\boldsymbol{m}) = (\boldsymbol{n},\boldsymbol{n}+\boldsymbol{e}_{i+s-1,i}), (\boldsymbol{n},\boldsymbol{n}+\boldsymbol{e}_{i+s,i+1}), (\boldsymbol{n}+\boldsymbol{e}_{i+1,i},\boldsymbol{n}+\boldsymbol{e}_{i+s,i}), (\boldsymbol{n}+\boldsymbol{e}_{i+1,i},\boldsymbol{n}+\boldsymbol{e}_{i+s,i})$. If we further assume that the populations evolve much more slowly than $\gamma_{\rm sp}^{-1}$, we can pull the source term out of the integral in Eq. (5) and obtain

$$\rho_{\boldsymbol{n}}^{\boldsymbol{n}+\boldsymbol{e}_{i+s,i}}(t) \simeq \rho_{\boldsymbol{n}}^{\boldsymbol{n}+\boldsymbol{e}_{i+s,i}}(0)\mathrm{e}^{-\lambda_{i+s,i}t} + \frac{JS_{i+s,i}(t)}{U(n_{i+s}-n_i+1)-\mathrm{i}\hbar\gamma_{\rm sp}}\big(1-\mathrm{e}^{-\lambda_{i+s,i}t}\big). \tag{6}$$

For $\gamma_{\rm sp}t \gg 1$, the slow component

$$\left(\rho_{\boldsymbol{n}}^{\boldsymbol{n}+\boldsymbol{e}_{i+s,i}}\right)_{\rm slow} \simeq \frac{J\sqrt{n_i(n_{i+s}+1)}\,S_{i+s,i}(t)}{U(n_{i+s}-n_i+1)-\mathrm{i}\hbar\gamma_{\rm sp}}. \tag{7}$$

acts as a slave variable depending on the slowly-evolving populations.

Applying this logic to the $s=1$ coherence, one finds that the source term depends only on the difference of the populations $\pi_{\boldsymbol{n}}$ and $\pi_{\boldsymbol{n}+\boldsymbol{e}_{i+1,i}}$,

$$S_{i+1,i} \approx \sqrt{n_i(n_{i+1}+1)}\,\big(\pi_{\boldsymbol{n}} - \pi_{\boldsymbol{n}+\boldsymbol{e}_{i+1,i}}\big). \tag{8}$$

The slow component reads

$$\left(\rho_{\boldsymbol{n}}^{\boldsymbol{n}+\boldsymbol{e}_{i+1,i}}\right)_{\rm slow} \simeq \frac{J\sqrt{n_i(n_{i+1}+1)}\,\big(\pi_{\boldsymbol{n}} - \pi_{\boldsymbol{n}+\boldsymbol{e}_{i+1,i}}\big)}{U(n_{i+1}-n_i+1)-\mathrm{i}\hbar\gamma_{\rm sp}}. \tag{9}$$

Substituting the slow component in Eq. (2) yields a coarse-grained (on a time scale $\gg \gamma_{\rm sp}^{-1}$) evolution equation for the Fock state populations $\pi_{\boldsymbol{n}}$ (see Eq. (3S) in the Supplementary Material of [2]).

An additional simplification comes from assuming a factorization ansatz for the dominant part of the density matrix,

$$\hat\rho = \prod_i \hat\rho_i. \tag{10}$$

We introduce the on-site number distribution $p_n$ by $p_{n_i} = \langle n_i|\hat\rho_i|n_i\rangle$ the diagonal elements, with $\sum_{n=0}^{\infty} p_n = 1$. The equation governing the evolution of the populations then reduces to the classical master equation (13) in the main article.

## II. SINGLE-PARTICLE CORRELATION FUNCTION

### A. Asymptotic behavior of $C_s$ for $\gamma_{\rm sp}t \gg 1$ and $s = 1, 2$

We compute the normalized single-particle correlator,

$$C_s(t) = \frac{1}{N}\sum_i \langle \hat a_{i+s}^\dagger \hat a_i\rangle = \frac{1}{N}\sum_i\sum_{\boldsymbol{n}} \sqrt{n_i(n_{i+s}+1)}\rho_{\boldsymbol{n}+\boldsymbol{e}_{i+s}-\boldsymbol{e}_i}^{\boldsymbol{n}}. \tag{11}$$

Using Eq. (7) and $C_{-s} = C_s^*$, we obtain the coarse-grained approximation of the correlator in the asymptotic regime,

$$C_s(t) \simeq \frac{J}{2U\bar nN_{\rm s}}\sum_i\sum_{\boldsymbol{n}}\sqrt{n_i(n_{i+s}+1)}\,\mathrm{Re}\frac{S_{i+s,i}^*(t)}{n_{i+s}-n_i+1+\mathrm{i}\varepsilon\bar n}\cdot\left(\rho_{\boldsymbol{n}}^{\boldsymbol{n}} - \rho_{\boldsymbol{n}+\boldsymbol{e}_{i\pm1,i}}^{\boldsymbol{n}+\boldsymbol{e}_{i\pm1,i}}\right). \tag{12}$$

In accordance with the approximations made to obtain Eq. (7), the source term $S_{i+s,i}$ in Eq. (12) only contains terms involving coherences of order $s-1$.

Using Eq. (8), the nearest-neighbors correlator with $s=1$ is given by

$$C_1(t) \simeq \frac{J}{U\bar{n}} \frac{1}{N_{\mathrm{s}}} \sum_i \sum_{\boldsymbol{n}} \frac{n_i(n_{i+s}+1)(n_{i+s}-n_i+1)}{(n_{i+s}-n_i+1)^2+(\varepsilon\bar{n})^2} \Big(\pi_{\boldsymbol{n}} - \pi_{\boldsymbol{n}+\boldsymbol{e}_{i+1,i}}\Big). \tag{13}$$

We now use the factorized approximation (10), which implies $\pi_{\boldsymbol{n}} = \prod_i p_{n_i}$. We get

$$C_1(t) \simeq \frac{1}{N_{\mathrm{s}}} \sum_i \prod_{k\neq i,i+1} \left(\sum_{n_k=0}^{+\infty} p_{n_k}\right) \frac{J}{U\bar{n}} \sum_{n_i,n_{i+1}=0}^{+\infty} \frac{n_i(n_{i+s}+1)(n_{i+s}-n_i+1)}{(n_{i+s}-n_i+1)^2+(\varepsilon\bar{n})^2} \big(p_{n_i}p_{n_{i+1}} - p_{n_i-1}p_{n_{i+1}+1}\big). \tag{14}$$

Since $\sum_{n_k} p_{n_k} = 1$ and since all the terms in the sum over sites $i$ are identical, we find Eq. (19) in the main article after relabeling the indices as $n_i = n$ and $n_{i+1} = m$.

For the nearest-neighbors correlator with $s=2$, we also start from Eq. (12,7) and evaluate the source term in the numerator keeping only the terms proportional to $s=1$ coherences. We obtain a rather bulky and not particularly illuminating expression of $C_2(\tau)$ in terms of the populations $\rho_{\boldsymbol{m}}^{\boldsymbol{m}}$ with $\boldsymbol{m} = \boldsymbol{n}, \boldsymbol{n}+\boldsymbol{e}_{i+1}-\boldsymbol{e}_i, \boldsymbol{n}+\boldsymbol{e}_{i+2}-\boldsymbol{e}_{i+1}, \cdots$. We also use the factorization ansatz Eq. (10) and follow the same general method as for $C_1$. We omit the details of the rather lengthy algebra, and only quote the final expression for $C_2$,

$$\begin{aligned} C_2(\tau) = \left(\frac{J}{U}\right)^2 \sum_{m,n,q} & \frac{mn(q+1)}{(q-m+1+\mathrm{i}\varepsilon\bar{n})(q-n+1+\mathrm{i}\varepsilon\bar{n})} \Big(p_n p_q - p_{n-1}p_{q+1}\Big)\Big(p_m - p_{m-1}\Big) \\ &+ \frac{m(n+1)(q+1)}{(q-m+1+\mathrm{i}\varepsilon\bar{n})(n-m+1+\mathrm{i}\varepsilon\bar{n})} \Big(p_m p_n - p_{m-1}p_{n+1}\Big)\Big(p_q p_{q+1}\Big). \end{aligned} \tag{15}$$

### B. Calculation of $C_1, C_2$ in the scaling limit

Analytical results can be obtained by taking the continuum $\bar{n} \to +\infty$ and scaling $\varepsilon \to 0$ limits. We first consider the continuum limit, where the discrete variables (*e.g.* $m$) and distributions ($p_m$) are promoted to continuous ones, $m \to x = \delta m$, $p_m \to \delta p(x)$, with $\delta = 1/\bar{n} \to 0$. Note that the normalization of the distribution is preserved, $\sum_m p_m = 1 \to \int dx p(x) = 1$ with $dx \equiv \delta$. After some algebra, we obtain

$$C_1(\tau) = \frac{J}{U\bar{n}} \int_{\mathbb{R}_+^2} dx dx' \, \frac{xx'(x'-x)}{(x'-x)^2+\varepsilon^2} \Big[\partial_x p(x) p(x') - p(x)\partial_{x'}p(x')\Big], \tag{16}$$

$$\begin{aligned} C_2(\tau) = \left(\frac{J}{U\bar{n}}\right)^2 \int dx dx' dx'' \frac{xx'x''}{(x''-x)^2+\varepsilon^2} & \Bigg[\frac{(x''-x)(x'-x)-\varepsilon^2}{(x'-x)^2+\varepsilon^2} \Big(p(x)\partial_{x'}p(x') - \partial_x p(x) p(x')\Big)\partial_z p(z) \\ &+ \frac{(x''-x)(x''-x')-\varepsilon^2}{(x''-x')^2+\varepsilon^2} \partial_x p(x) \Big(\partial_{x'}p(x')p(x'') - p(x')\partial_{x''}p(x'')\Big)\Bigg]. \end{aligned} \tag{17}$$

We omitted the argument $\tau$ in the distribution function to lighten notations.

We take next the scaling limit $\varepsilon \to 0$. The distribution function becomes $p(x,\tau) = \tau^{-\beta} f(u)$, with $u = (x-1)/\tau^{1/4}$ the scaling variable and $f(u)$ the scaling function. We change to scaled variables $(x, x', x'') \to (u = (x-1)/\tau^{1/4}, v = (x'-1)/\tau^{1/4}, w = (x''-1)/\tau^{1/4})$ and consider short rescaled times $\tau \ll 1$. In this regime, we may substitute $x \approx x' \approx x'' \approx 1$ for the variables appearing alone in the numerator. This approximation yields the scaling forms

$$C_1(t) \underset{\varepsilon\to 0}{\longrightarrow} a_1 \frac{J}{U\bar{n}\tau^{2\beta}} = \frac{a_1}{\sqrt{2z\gamma_{\mathrm{sp}}t}}, \tag{18}$$

$$C_2(t) \underset{\varepsilon\to 0}{\longrightarrow} a_2 \left(\frac{J}{U\bar{n}}\right)^2 = \frac{a_2}{2z\gamma_{\mathrm{sp}}t}, \tag{19}$$

with numerical factors

$$a_1 = \int_{\mathbb{R}^2} dudv \, \frac{f'(u)f(v) - f(u)f'(v)}{v-u} f(u)f(v), \tag{20}$$

$$a_2 = \frac{1}{16} \int_{\mathbb{R}^3} dudvdw \, \frac{1}{w-u} \left[ \frac{w^3(u^3-v^3)}{u-v} - \frac{u^3(w^3-v^3)}{w-v} \right] f(u)f(v)f(w). \tag{21}$$

The true scaling function $f_\infty$ corresponds to $a_1^\infty = 2\Gamma\left(\frac{3}{4}\right)/\Gamma\left(\frac{1}{4}\right) \approx 0.676\cdots$ and $a_2^\infty = 3\left(a_1^\infty\right)^2/4 \approx 0.343$, with $\Gamma$ the Euler gamma function. Using the Gaussian scaling distribution $f_{\mathrm{approx}}$ relevant for finite $\bar{n}$ (see Section IV in the main article ), we find instead $a_1 = a_2 \approx 1$.


[1] D. Poletti, J.-S. Bernier, A. Georges, and C. Kollath, Physical Review Letters **109**, 045302 (2012), URL `https://link.aps.org/doi/10.1103/PhysRevLett.109.045302`.

[2] D. Poletti, P. Barmettler, A. Georges, and C. Kollath, Physical Review Letters **111**, 195301 (2013), URL `https://link.aps.org/doi/10.1103/PhysRevLett.111.195301`.
